# Supplementary material for: ReDirTrans: Latent-to-Latent Translation for Gaze and Head Redirection
Source: arXiv:2305.11452 source file (2023-05-19)
Supplement: Supplementary file 1 [file 6-appendix.tex]

\appendix
\label{sec:appendix}

\section{Overview}
In this supplementary document, first, we demonstrate training details when we incorporate ReDirTrans with encoder-generator pair. 
Then we present some additional quantitative results of ReDirTrans-GAN. 
Lastly, we introduce the details when we implemented other state-of-the-art baselines. 

\section{Implementation Details}
We trained and evaluated ReDirTrans given two different encoder-generator pairs: 1) the trainable encoder-decoder pair from ST-ED \cite{zheng2020self}; 2) the pre-trained e4e \cite{tov2021designing} and StyleGAN \cite{karras2020analyzing}.
Thus we introduced implementation details in two cases: 1) \textit{ReDirTrans} and 2) \textit{ReDirTrans-GAN}. 

\subsection{Datasets}
GazeCapture \cite{krafka2016eye} is the largest public gaze-related full-face dataset including $1,474$ participants with over two million frames taken under unconstrained scenarios. 
We utilize its training subset to train the redirector and evaluate the redirection precision with its test subset. 
 
MPIIFaceGaze \cite{zhang2017s} is a widely used benchmark dataset for the in-the-wild gaze estimation task. 
It includes $37,667$ full-face images captured from $15$ participants with varied head orientations, multiple gaze directions and different illuminations. 
We utilize this dataset to evaluate the cross-dataset redirection performance. 

CelebA-HQ \cite{karras2017progressive} is a high-quality version of CelebA \cite{liu2015deep} that consists of $30,000$ images at 1024×1024 resolution. 
We utilize this dataset for evaluating the cross-dataset qualitative redirection performance. 

\subsection{Preprocessing Steps}
1) \textit{ReDirTrans}: We preprocessed the image data to acquire a $128\times128$ restricted range of face images aligned with key points of the nose and eyes, followed by \cite{zheng2020self}. 

2) \textit{ReDirTrans-GAN}: We preprocessed the image data to acquire $256\times256$ full-face images aligned with key points of the mouth and eyes. 
We utilized reflective padding to the blank areas after alignment and then covered these areas with Gaussian blur, followed by \cite{karras2017progressive}. 

\subsection{Projector-Deprojector}
% Given the input latent vectors encoded from images, we further project them into an interpretable space to achieve transformation equivariant mappings between this embedding space and image space. 
Since the inputs to the projector have already been the decoded latent vectors from images, we utilized several fully connected modules as the architectures of the projector-deprojector. 
1) \textit{ReDirTrans}: Unlike ST-ED projecting the input latent vector into nine attribute embeddings, our proposed ReDirTrans only projected it into the aimed attribute (gaze directions and head orientations) embeddings. 
The size of the estimated label and embedding of one attribute are $2$ and $3\times 16$, respectively. 
The details are illustrated in Table \ref{tab:arch_P_DP}.

1) \textit{ReDirTrans-GAN}: As for the ReDirTrans-GAN, the main difference comes from the size of latent vectors in latent space $\mathcal{F}$. 
The details are shown in Table \ref{tab:arch_P_DP_GAN}.

\begin{table}[t]
\begin{tabular}{@{}ccclll@{}}
\toprule
\multicolumn{2}{c}{\textbf{ReDirTrans}}     & \multicolumn{4}{c}{Layers/Blocks}                    \\ \midrule
\multirow{4}{*}{\textbf{P}} & \multirow{2}{*}{\begin{tabular}[c]{@{}c@{}}Pseudo \\ Label Branch\end{tabular}} & \multicolumn{4}{c}{FC(3072, 96, w/bias), LeakyReLU()}  \\
                   &                    & \multicolumn{4}{c}{FC(96, 4, w/bias), pi/2*Tanh()}   \\ \cmidrule(l){2-6} 
                   & \multirow{2}{*}{\begin{tabular}[c]{@{}c@{}}Embedding\\ Branch\end{tabular}}     & \multicolumn{4}{c}{FC(3072, 3072, w/bias), LeakyReLU()} \\
                   &                    & \multicolumn{4}{c}{FC(3072, 96, w/bias)}              \\ \midrule
\multicolumn{2}{c}{\multirow{2}{*}{\textbf{DP}}} & \multicolumn{4}{c}{FC(96, 1024, w/bias), LeakyReLU()} \\ 
\multicolumn{2}{c}{}                    & \multicolumn{4}{c}{FC(1024, 3072, w/bias)} \\
\bottomrule
\end{tabular}
\caption{The architecture of the projector and deprojector in \textbf{ReDirTrans}. \textbf{P} denotes projector and \textbf{DP} denotes deprojector.}
\label{tab:arch_P_DP}
\end{table}

\begin{table}[t]
\begin{tabular}{@{}ccclll@{}}
\toprule
\multicolumn{2}{c}{\textbf{ReDirTrans-GAN}}     & \multicolumn{4}{c}{Layers/Blocks}                    \\ \midrule
\multirow{4}{*}{\textbf{P}} & \multirow{2}{*}{\begin{tabular}[c]{@{}c@{}}Pseudo \\ Label Branch\end{tabular}} & \multicolumn{4}{c}{FC(512, 64, w/bias), LeakyReLU()}  \\
                   &                    & \multicolumn{4}{c}{FC(64, 4, w/bias), pi/2*Tanh()}   \\ \cmidrule(l){2-6} 
                   & \multirow{2}{*}{\begin{tabular}[c]{@{}c@{}}Embedding\\ Branch\end{tabular}}     & \multicolumn{4}{c}{FC(512, 128, w/bias), LeakyReLU()} \\
                   &                    & \multicolumn{4}{c}{FC(128, 96, w/bias)}              \\ \midrule
\multicolumn{2}{c}{\multirow{2}{*}{\textbf{DP}}} & \multicolumn{4}{c}{FC(96, 256, w/bias), LeakyReLU()} \\
\multicolumn{2}{c}{}                    & \multicolumn{4}{c}{FC(256, 512, w/bias)}             \\ \bottomrule
\end{tabular}
\caption{The architecture of the projector and deprojector in \textbf{ReDirTrans-GAN}. \textbf{P} denotes projector and \textbf{DP} denotes deprojector.}
\label{tab:arch_P_DP_GAN}
\end{table}

\subsection{Encoder-Generator and Loss Functions}
1) \textit{ReDirTrans}: ST-ED proposed the architecture of encoder-decoder pair given the DenseNet \cite{huang2017densely} architecture, for $128\times 128$ output. 
As for the decoder, the convolutional layers were replaced by the transposed convolutional layers and the average-pooling layers. 
The detailed encoder-decoder structure is illustrated in \cite{zheng2020self}. 
To ensure the generation quality, we utilized a PatchGAN \cite{isola2017image} discriminator with corresponding adversarial loss as proposed in ST-ED during the training. 

2) \textit{ReDirTrans-GAN}: Since both e4e and StyleGAN were pretrained and fixed during the training, the image discriminator mentioned above was no longer used. 
Instead, to maintain the perceptual quality and editability of latent codes after redirection as the original latent codes encoded by e4e, we kept utilizing the e4e proposed delta-regularization loss $\mathcal{L}_{d-reg}$ and the adversarial loss $\mathcal{L}_{adv}$ by a latent discriminator \cite{nitzan2020face}. 
Noted that we applied these two loss functions to the modified latent vectors after redirection to maintain the editability of e4e encoded latent vectors. 

\subsection{Gaze and Head Pose Estimation Network}
During training, we need a pretrained gaze and head pose estimation network $\xi_{hg}(\cdot)$ as the estimator to supervise the redirection process.
During the evaluation, we require another different external pretrained gaze and head pose estimation network $\xi^\prime_{hg}(\cdot)$, which is unseen during training, to evaluate the consistency of the aimed attributes between redirected and target samples. 
We followed the pipeline proposed by ST-ED, which utilized a VGG-16-based $\xi_{hg}(\cdot)$ \cite{simonyan2014very} and a ResNet50-based $\xi^\prime_{hg}(\cdot)$ \cite{he2016deep}. 

1) \textit{ReDirTrans}: We retrained and employed the VGG-16-based $\xi_{hg}(\cdot)$ and ResNet50-based $\xi^\prime_{hg}(\cdot)$ as the gaze and head pose estimators, given the architectures and training parameters illustrated in \cite{zheng2020self}.

2) \textit{ReDirTrans-GAN}: To fit the different sizes of input ($256\times256$) and output images ($1024\times1024$) with the full face range when training and evaluating ReDirTrans-GAN, we downsampled the output images to $256\times256$. 
The fully connected modules after the convolutional part of $\xi_{hg}(\cdot)$ and $\xi^\prime_{hg}(\cdot)$ were modified accordingly for different input sizes compared with the ST-ED version. 
The detailed structures of $\xi_{hg}(\cdot)$ and $\xi^\prime_{hg}(\cdot)$ are shown in Table \ref{sup_tab:vgg16} and Table \ref{sup_tab:res50}, respectively. 

\begin{table}[t]
\centering
\begin{tabular}{@{}cc@{}}
\toprule
\textbf{Nr.} & \textbf{layers / blocks}                                           \\ \midrule
0            & VGG-16 Conv layers                                        \\
1            & AvgPool2d(size=4, stride=4)                                        \\
2            & FC(2048, 128, w/bias), LeakyReLU()                                 \\
3            & FC(128, 64, w/bias), LeakyReLU()                                   \\
4            & FC(64, 4, w/bias), $0.5\pi\cdot \tanh()$ \\ \bottomrule
\end{tabular}
\caption{The architecture of the VGG-16-based gaze direction and head orientation estimation network, $\xi_{hg}(\cdot)$. }
\label{sup_tab:vgg16}
\end{table}

\begin{table}[t]
\centering
\begin{tabular}{@{}cc@{}}
\toprule
\textbf{Nr.} & \textbf{layers / blocks}                                         \\ \midrule
0   & ResNet-50 Conv layers, stride of MaxPool2d=1 \\
1   & FC(2048, 4, w/bias)                                     \\ \bottomrule
\end{tabular}
\caption{The architecture of the ResNet50-based gaze direction and head orientation estimation network, $\xi^\prime_{hg}(\cdot)$. }
\label{sup_tab:res50}
\end{table}

\subsection{Training Hyperparameters} 
1) \textit{ReDirTrans}: We trained ReDirTrans and the encoder-decoder pair with the same hyperparameters as ST-ED \cite{zheng2020self} by using over $1.4\times10^6$ full-face images from GazeCapture Training subset. 

2) \textit{ReDirTrans-GAN}: We randomly chose $10,000$ images from the GazeCapture training subset to train ReDirTrans-GAN since both the encoder and generator are fixed and pretrained. 
The number of epochs is $2$ with a batch size of $2$. 
The initial learning rate is $10^{-4}$ and is decayed by $0.8$ every $3,000$ iterations. 
The optimizer is Adam \cite{kingma2014adam} with the default momentum value of $\beta_1=0.9,\beta_2=0.999$. 

The loss weights are $\lambda_{r}=8$, $\lambda_{L}=8$, $\lambda_{ID}=5$, $\lambda_{a}=1$, $\lambda_{l}=5$, $\lambda_{e}=2$, $\lambda_{p}=10$, $\lambda_{d-reg}=0.0002$, $\lambda_{adv}=2$, where $\lambda_{d-reg}$ and $\lambda_{adv}$ are the weights of delta-regularization loss $\mathcal{L}_{d-reg}$ and the adversarial loss $\mathcal{L}_{adv}$, respectively. 

\subsection{Redirection Step}
% Rotation Matrix
We applied rotation matrices built by the pitch and yaw to the estimated embeddings for redirection purposes. 
\begin{equation}
    \begin{bmatrix}
    \cos \phi^i & 0 & \sin\phi^i \\ 
    0 & 1 & 0 \\ 
    -sin\phi^i & 0 & \cos\phi^i
    \end{bmatrix}
\cdot
    \begin{bmatrix}
    1 & 0 & 0 \\
    0 & \cos\theta^i & -\sin\theta^i \\
    0 & \sin\theta^i & cos\theta^i
    \end{bmatrix}, i\in\{1, 2\}
\end{equation}
where $\phi$ represents yaw and $\theta$ represents pitch, and index $i\in\{1, 2\}$ represents gaze directions and head orientations, respectively.  

\input{1-tables/sup_tab:correct.tex}

\section{Further Results}
\subsection{Gaze Correction}
Table \ref{tab:correction_GC} and Table \ref{tab:correction_celeb} present within- and cross-dataset evaluation performance for gaze correction tasks. 
e4e inversion results can maintain gaze directions and head orientations better in CelebA-HQ than GazeCapture since samples in CelebA-HQ have much less varied gaze directions and head orientations. 
However, after we included ReDirTrans in the inversion pipeline as ReDirTrans-GAN, we can successfully maintain gaze directions and head orientations without affecting identity information (ID), which was measured by a pretrained ArcFace model \cite{deng2019arcface}. 
Fig. \ref{sup_fig:correct} shows several examples. 

\subsection{Redirection Accuracy of ReDirTrans-GAN}
Table \ref{tab:rediretrans-gan_results} presents the redirection accuracy of ReDirTrans-GAN in the GazeCapture test subset. 
We can observe that ReDirTrans-GAN cannot achieve as accurate redirection performance as ReDirTrans, which worked with the trainable encoder-decoder pair. 
There exists a \textbf{trade-off} between redirection accuracy and the following considerations:
\vspace{-0.2cm}
\begin{itemize}
\itemsep 0em
\item We utilized \underline{fixed} encoder and generator parameters during the redirector training to ensure no modification to the predefined latent space; 
\item e4e encoded latent vectors in $W^+$ have limitations to \underline{understanding gaze} in Section \ref{subsec:correction}. e4e was trained with the FFHQ dataset, which does not include samples with as varied gaze directions and head orientations as the samples in GazeCapture. 
Given some cases with large gaze directions or head orientations, e4e cannot invert them very well;
\item We kept the redirected latent codes within the `high editability space' proposed by e4e to allow for \underline{further editing} with other face editing techniques, sacrificing some quality (redirection accuracy); 
\item Extended face covering ranges and down-sampling of high-resolution generated images could cause the performance drop. 
\item The deprojector learned that the redirected latent vectors after addition and subtraction operations would not deviate away from the original input latent vectors. 
Thus ReDirTrans-GAN cannot redirect some extreme cases as well as ReDirTrans did, especially for head orientations.
\item Predefined face alignments (four eyes corners and two mouth corners) restricts both the encoder and generator's ability for extreme head pose synthesis. 
\end{itemize}
In summary, we made a deliberate choice to use a fixed encoder-generator pair, preserve edited latent codes in $W^+$, and edit within the `high editability space' to maintain compatibility with continuing facial attribute editing by other methods. 
ReDirTrans-GAN provides a solution to edit attributes in predefined feature spaces that have limited abilities to depict those attributes.
It also addresses the face editing task of redirecting or correcting gaze from the latent code perspective. 
Fig. \ref{sup_fig:redir_gaze} and Fig. \ref{sup_fig:redir_head} show redirected samples with modifying gaze directions and head orientations separately. 

\subsection{Layer-wise Weights}
Given the layer-wise representation of latent vectors in $W^+$ space, we proposed layer-wise weights loss to measure the contribution of each layer for the corresponding attribute redirection. 
We compared the redirected samples with and without considering the layer-wise weights loss, shown in Fig. \ref{sup_fig:redir_p}. 
We observed that gaze directions and head orientations become entangled without this loss and the network tends to learn a specific combination of gaze directions and head orientations. 
% However, if we utilize this loss with the estimated layer-wise weights to further modify each layer's output residuals, the gaze directions and head orientations can be disentangled and redirected independently. 
However, when we utilized this loss with the estimated layer-wise weights to modify each layer's output residuals further. 
In that case, gaze directions and head orientations can be disentangled and redirected independently.

\section{State-of-the-Art Baselines}
\subsection{ST-ED}
We preprocessed the face images as shown in ST-ED based on code repository \footnote{\url{https://github.com/swook/faze_preprocess}}. 
We trained and evaluated ST-ED based on their published code repository \footnote{\url{https://github.com/zhengyuf/STED-gaze}}.

\subsection{VecGAN}
VecGAN \cite{dalva2022vecgan} was originally proposed to modify facial attributes, such as gender, age, hair color, smiling and bangs. 
We applied the VecGAN's addition and subtraction operations in the latent space $\mathcal{F}$ to the ST-ED proposed encoder-decoder pair. 
Instead of estimating embeddings from input latent vectors, VecGAN only estimates the pseudo labels of the aimed attributes. 
We utilized four orthogonal global latent directions $1\times1344$ for pitch and yaw control of the gaze directions and head orientations separately. 
We cannot directly apply the estimated labels to the global latent directions in $\mathcal{F}$ by the multiplication operation due to the scale problem. 
Thus we applied a shallow network for transforming pseudo labels to scalars to fit for the global latent directions. 
The network structure is shown in Table \ref{sup_tab:trans}.

\begin{table}[t]
\centering
\begin{tabular}{@{}cc@{}}
\toprule
\textbf{Nr.} & \textbf{layers / blocks}                                         \\ \midrule
0   &   FC(4, 32, w/bias), LeakyReLU()  \\
1   &   FC(32, 64, w/bias), LeakyReLU() \\
2   &   FC(64, 64, w/bias), LeakyReLU() \\
3   &   FC(64, 4, w/bias) \\
\bottomrule
\end{tabular}
\caption{Architecture of the scale transformation network. This network transforms the pseudo labels into the scalars for the multiplication with the the global latent directions in $\mathcal{F}$.}
\label{sup_tab:trans}
\end{table}
